# Supplementary material for: Exploring Effective Mask Sampling Modeling for Neural Image Compression
Source: arXiv:2306.05704 source file (2023-06-09)

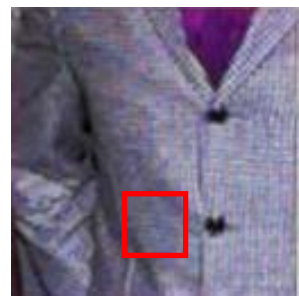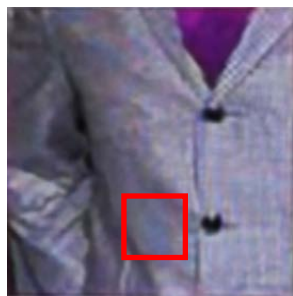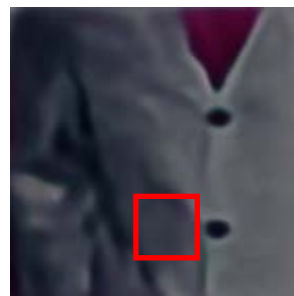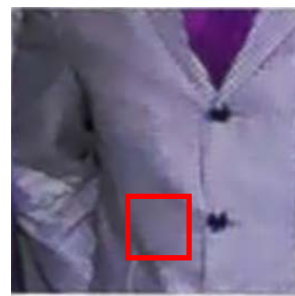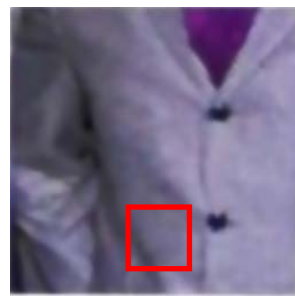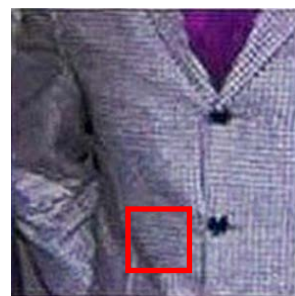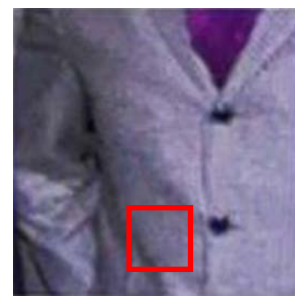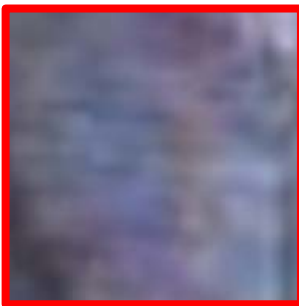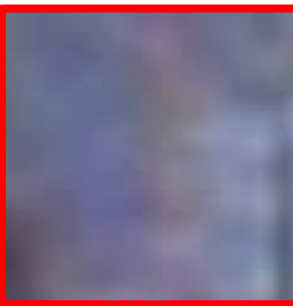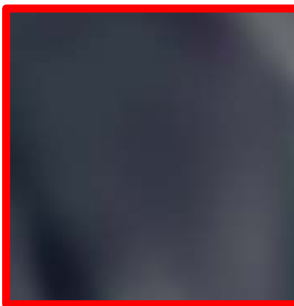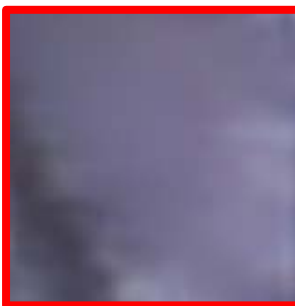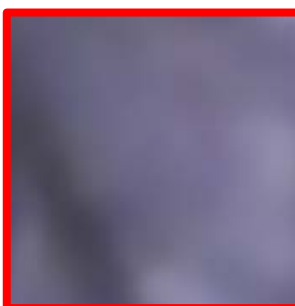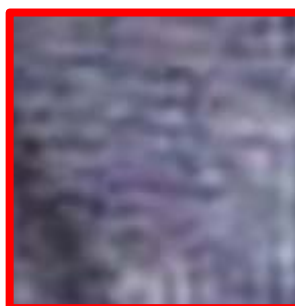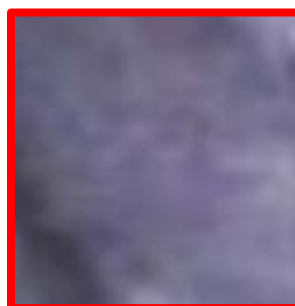

Moire image

DIP

Double-DIP

MSJF

GF

DJF

FDNet

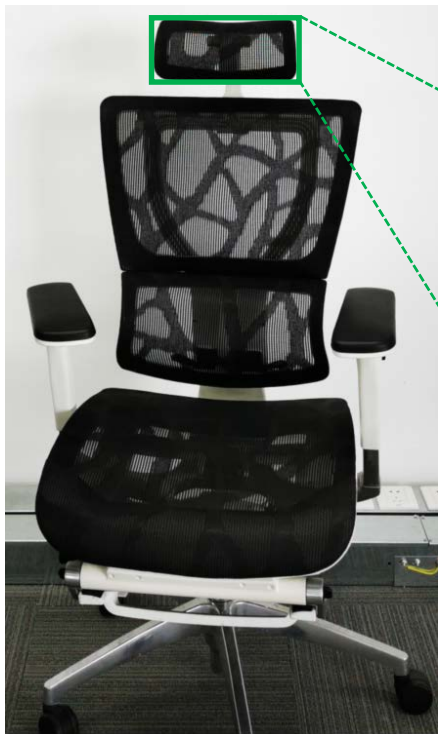

Focused image

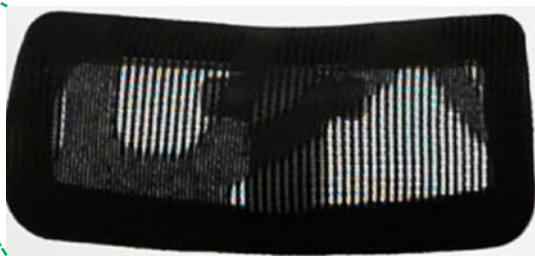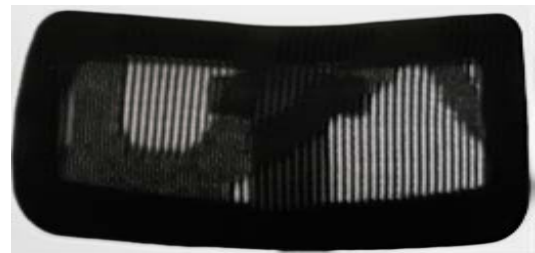

FDNet

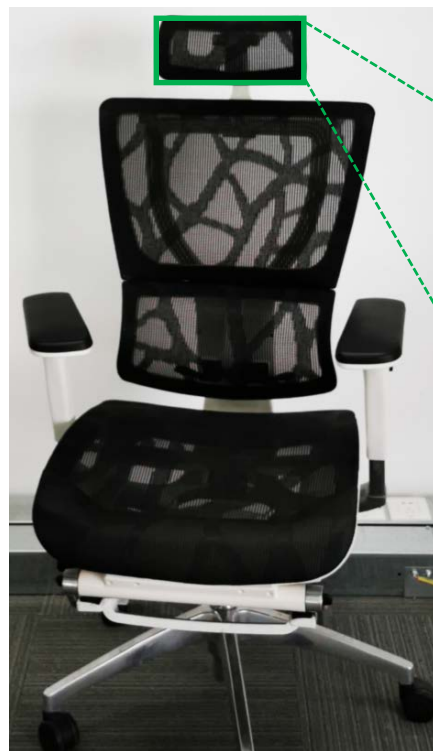

Defocused image

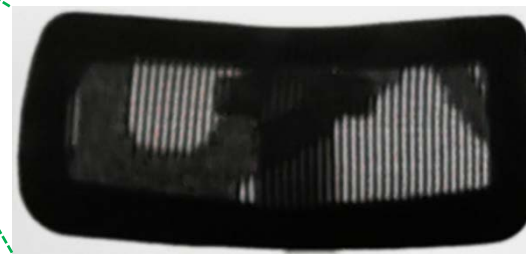

Supplement: Supplementary file 1 [file sample6_2.pdf]
